# Supplementary material for: SocialCircle+: Learning the Angle-based Conditioned Interaction Representation for Pedestrian Trajectory Prediction
Source: arXiv:2409.14984 source file (2024-09-23)
Supplement: Supplementary file 1 [file s3_partitions.tex]

%%%%%%%%%%%%%%%%%%%%%%%
%% Author: Conghao Wong
%% Date: 2023-10-08 11:02:46
%% LastEditors: Conghao Wong
%% LastEditTime: 2024-07-19 16:58:15
%% Description: file content
%% Github: https://cocoon2wong.github.io
%% Copyright 2023 Conghao Wong, All Rights Reserved.
%%%%%%%%%%%%%%%%%%%%%%%

\documentclass[../../paper.tex]{subfiles}

\begin{document}

\section{Additional Experimental Analyses on the Number of \EMODEL~Partitions}
\label{sec_appendix_partitions}

\TODO{Analyses of N_\theta in the Appendix}

\begin{table}[tbp]
    \small
    \centering
    \begin{tabular}{c|c|cc}
        \toprule
        Variations
        & $N_\theta$
        & ADE/FDE
        & Gain (\%) \\

        \midrule
        \VMODEL* & - & 7.04/10.94 & -4.92\%/-2.63\% \\
        \VMODEL-SC-a4 & 1 & 6.96/11.05 & -3.73\%/-3.66\% \\
        \VMODEL-SC-a5 & 4 & 6.79/10.80 & -1.19\%/-1.31\% \\
        \VMODEL-SC & 8 & 6.71/10.66 & (base) \\
        \VMODEL-SC-a6 & 12 & 6.65/10.60 & +0.89\%/+0.56\%\\
        \VMODEL-SC-a7 & 16 & 6.68/10.65 & +0.45\%/+0.09\%\\
        \VMODEL-SC-a8 & 36 & 6.64/10.64 & +1.04\%/+0.19\%\\

        \midrule
        \EVMODEL* & - & 6.73/10.75 & -2.91\%/-3.76\% \\
        \EVMODEL-SC-a4 & 1 & 6.66/10.70 & -1.83\%/-3.28\% \\
        \EVMODEL-SC-a5 & 4 & 6.61/10.55 & -1.07\%/-1.83\% \\
        \EVMODEL-SC & 8 & 6.54/10.36 & (base) \\
        \EVMODEL-SC-a6 & 12 & 6.50/10.34 & +0.61\%/+0.19\% \\
        \EVMODEL-SC-a7 & 16 & 6.46/10.22 & +1.22\%/+1.35\% \\
        \EVMODEL-SC-a8 & 36 & 6.57/10.41 & -0.46\%/-0.48\% \\
        
        \bottomrule
    \end{tabular}
    \caption{
        Ablation studies on verifying the number of \MODEL~partitions $N_\theta$ with different backbone models on SDD.
        Values in the ``Gain'' column are the percentage ADE and FDE gain compared to the base 8-partition model (denoted with ``(base)'').
    }
    \label{tab_ab_partitions}
\end{table}

\begin{figure}[t]
    \centering
    \includegraphics[width=1.0\linewidth]{../../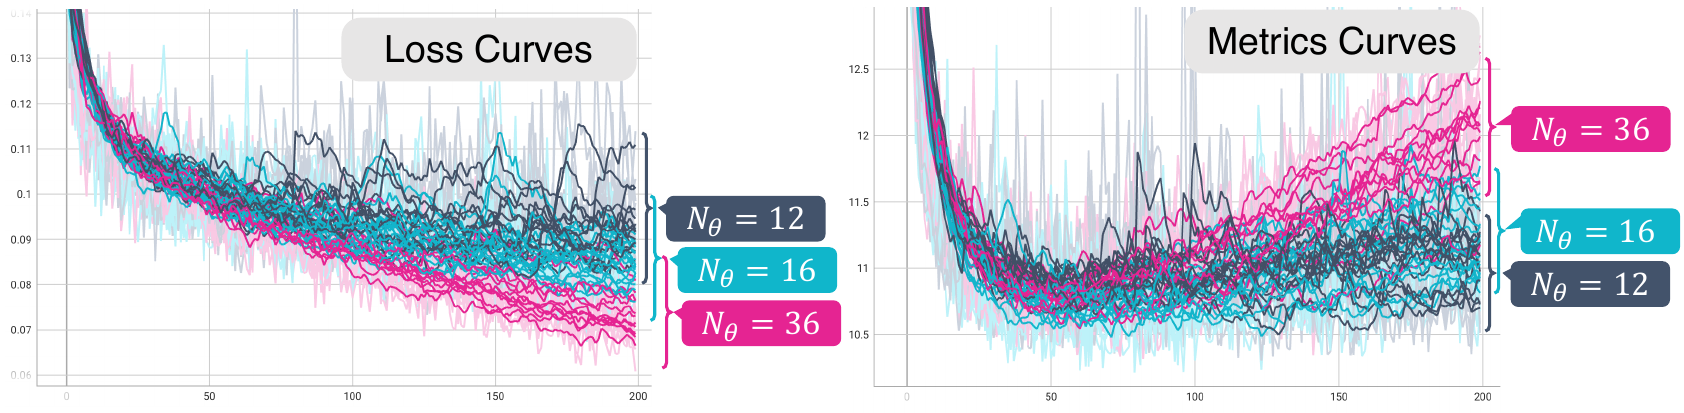}
    \caption{
        Loss curves (left, $\ell_2$ loss) and metrics curves (right, ADE) of \EVMODEL-SC variations a6 to a8 ($N_\theta \in \{12, 16, 36\}$).
    }
    \label{fig_loss_partitions}
\end{figure}

\begin{figure*}[t]
    \centering
    \includegraphics[width=1.0\linewidth]{../../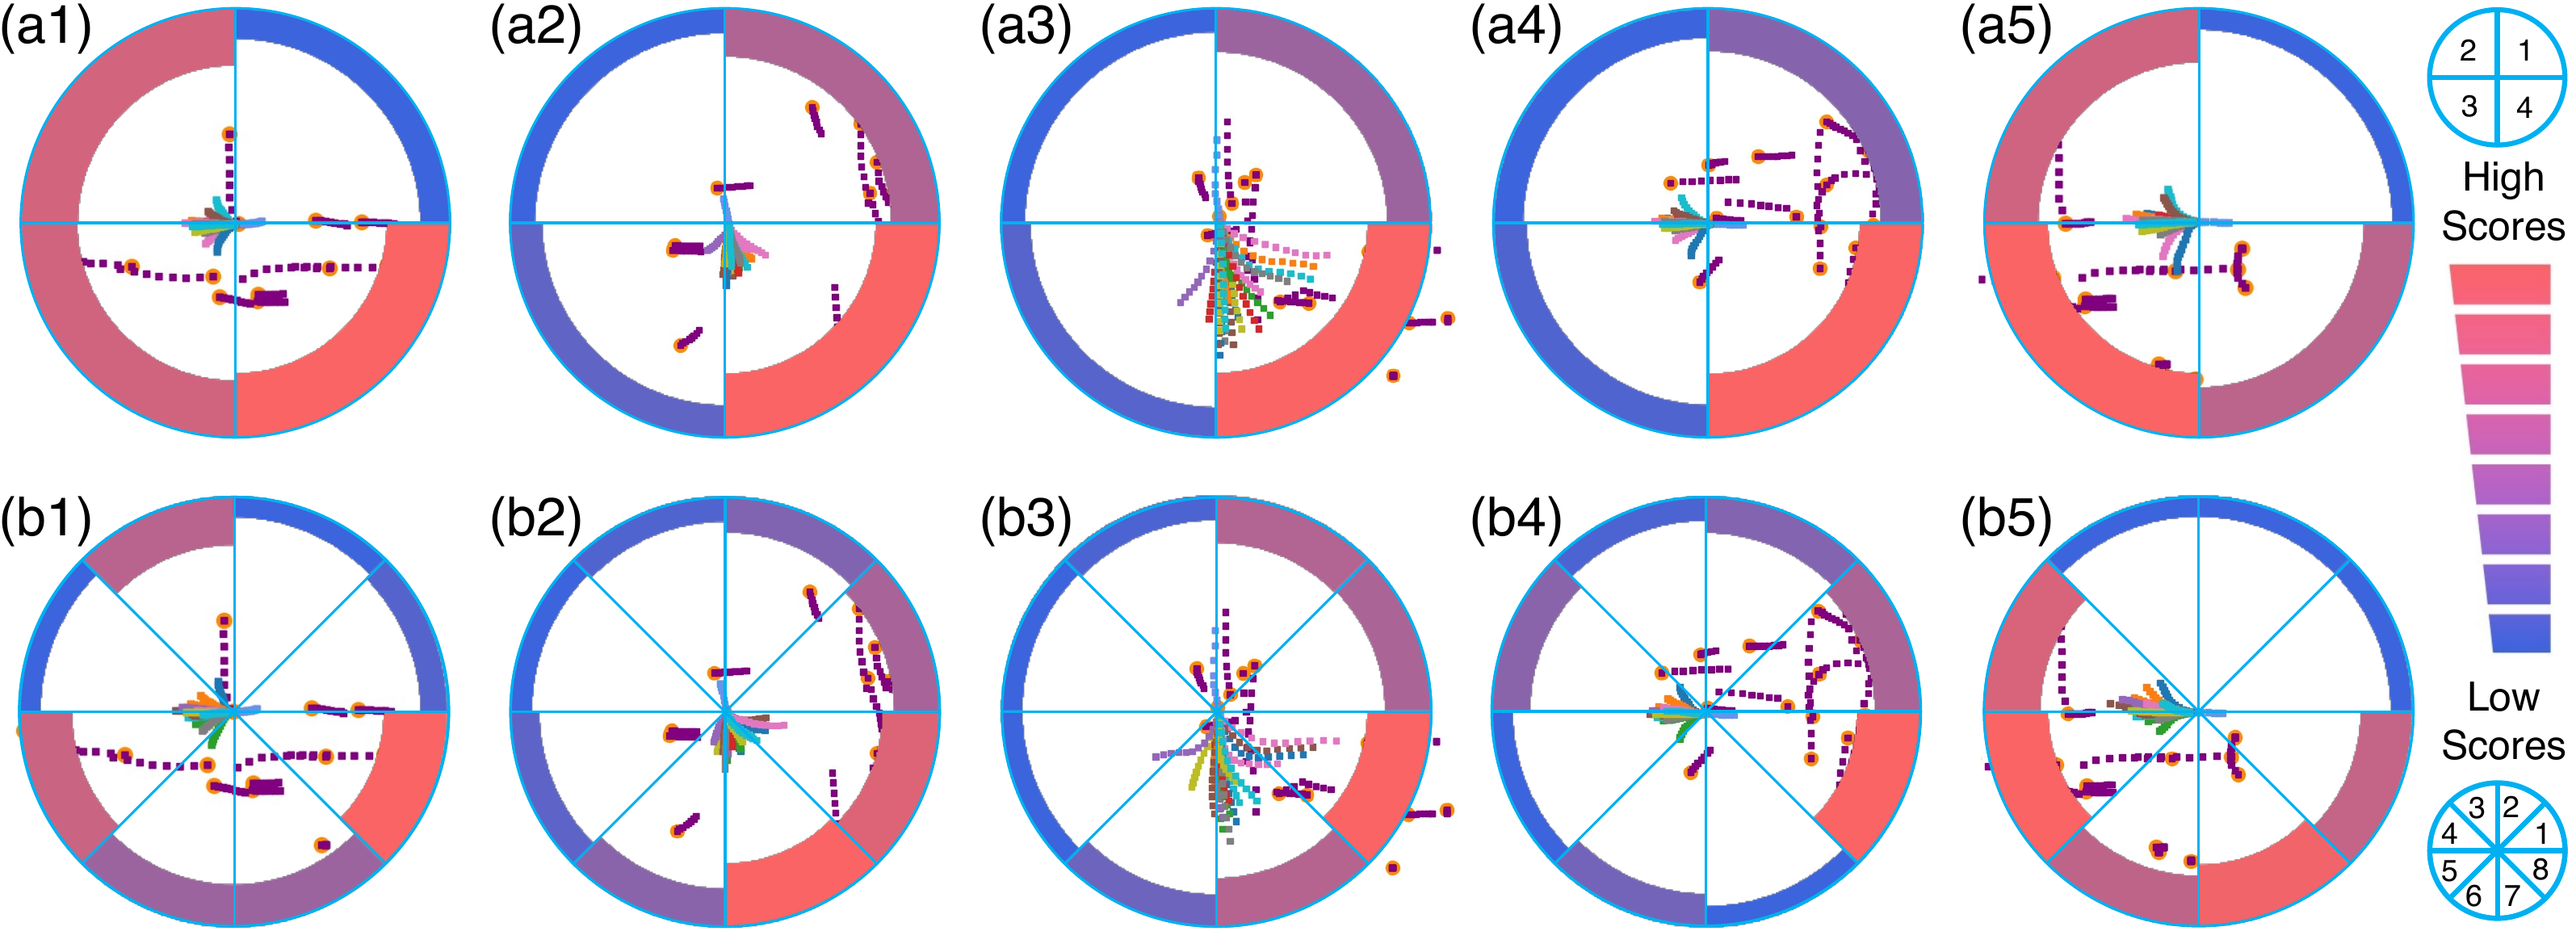}
    \caption{
        Visualized predicted trajectories and the corresponding attention scores of several real-world prediction cases on SDD-little0 provided by the \textbf{4-partition} \EVMODEL-SC (a1) to (a5) and the \textbf{8-partition} \EVMODEL-SC (b1) to (b5).
    }
    \label{fig_attention_partitions}
\end{figure*}

\begin{figure*}[t]
    \centering
    \includegraphics[width=0.916\linewidth]{../../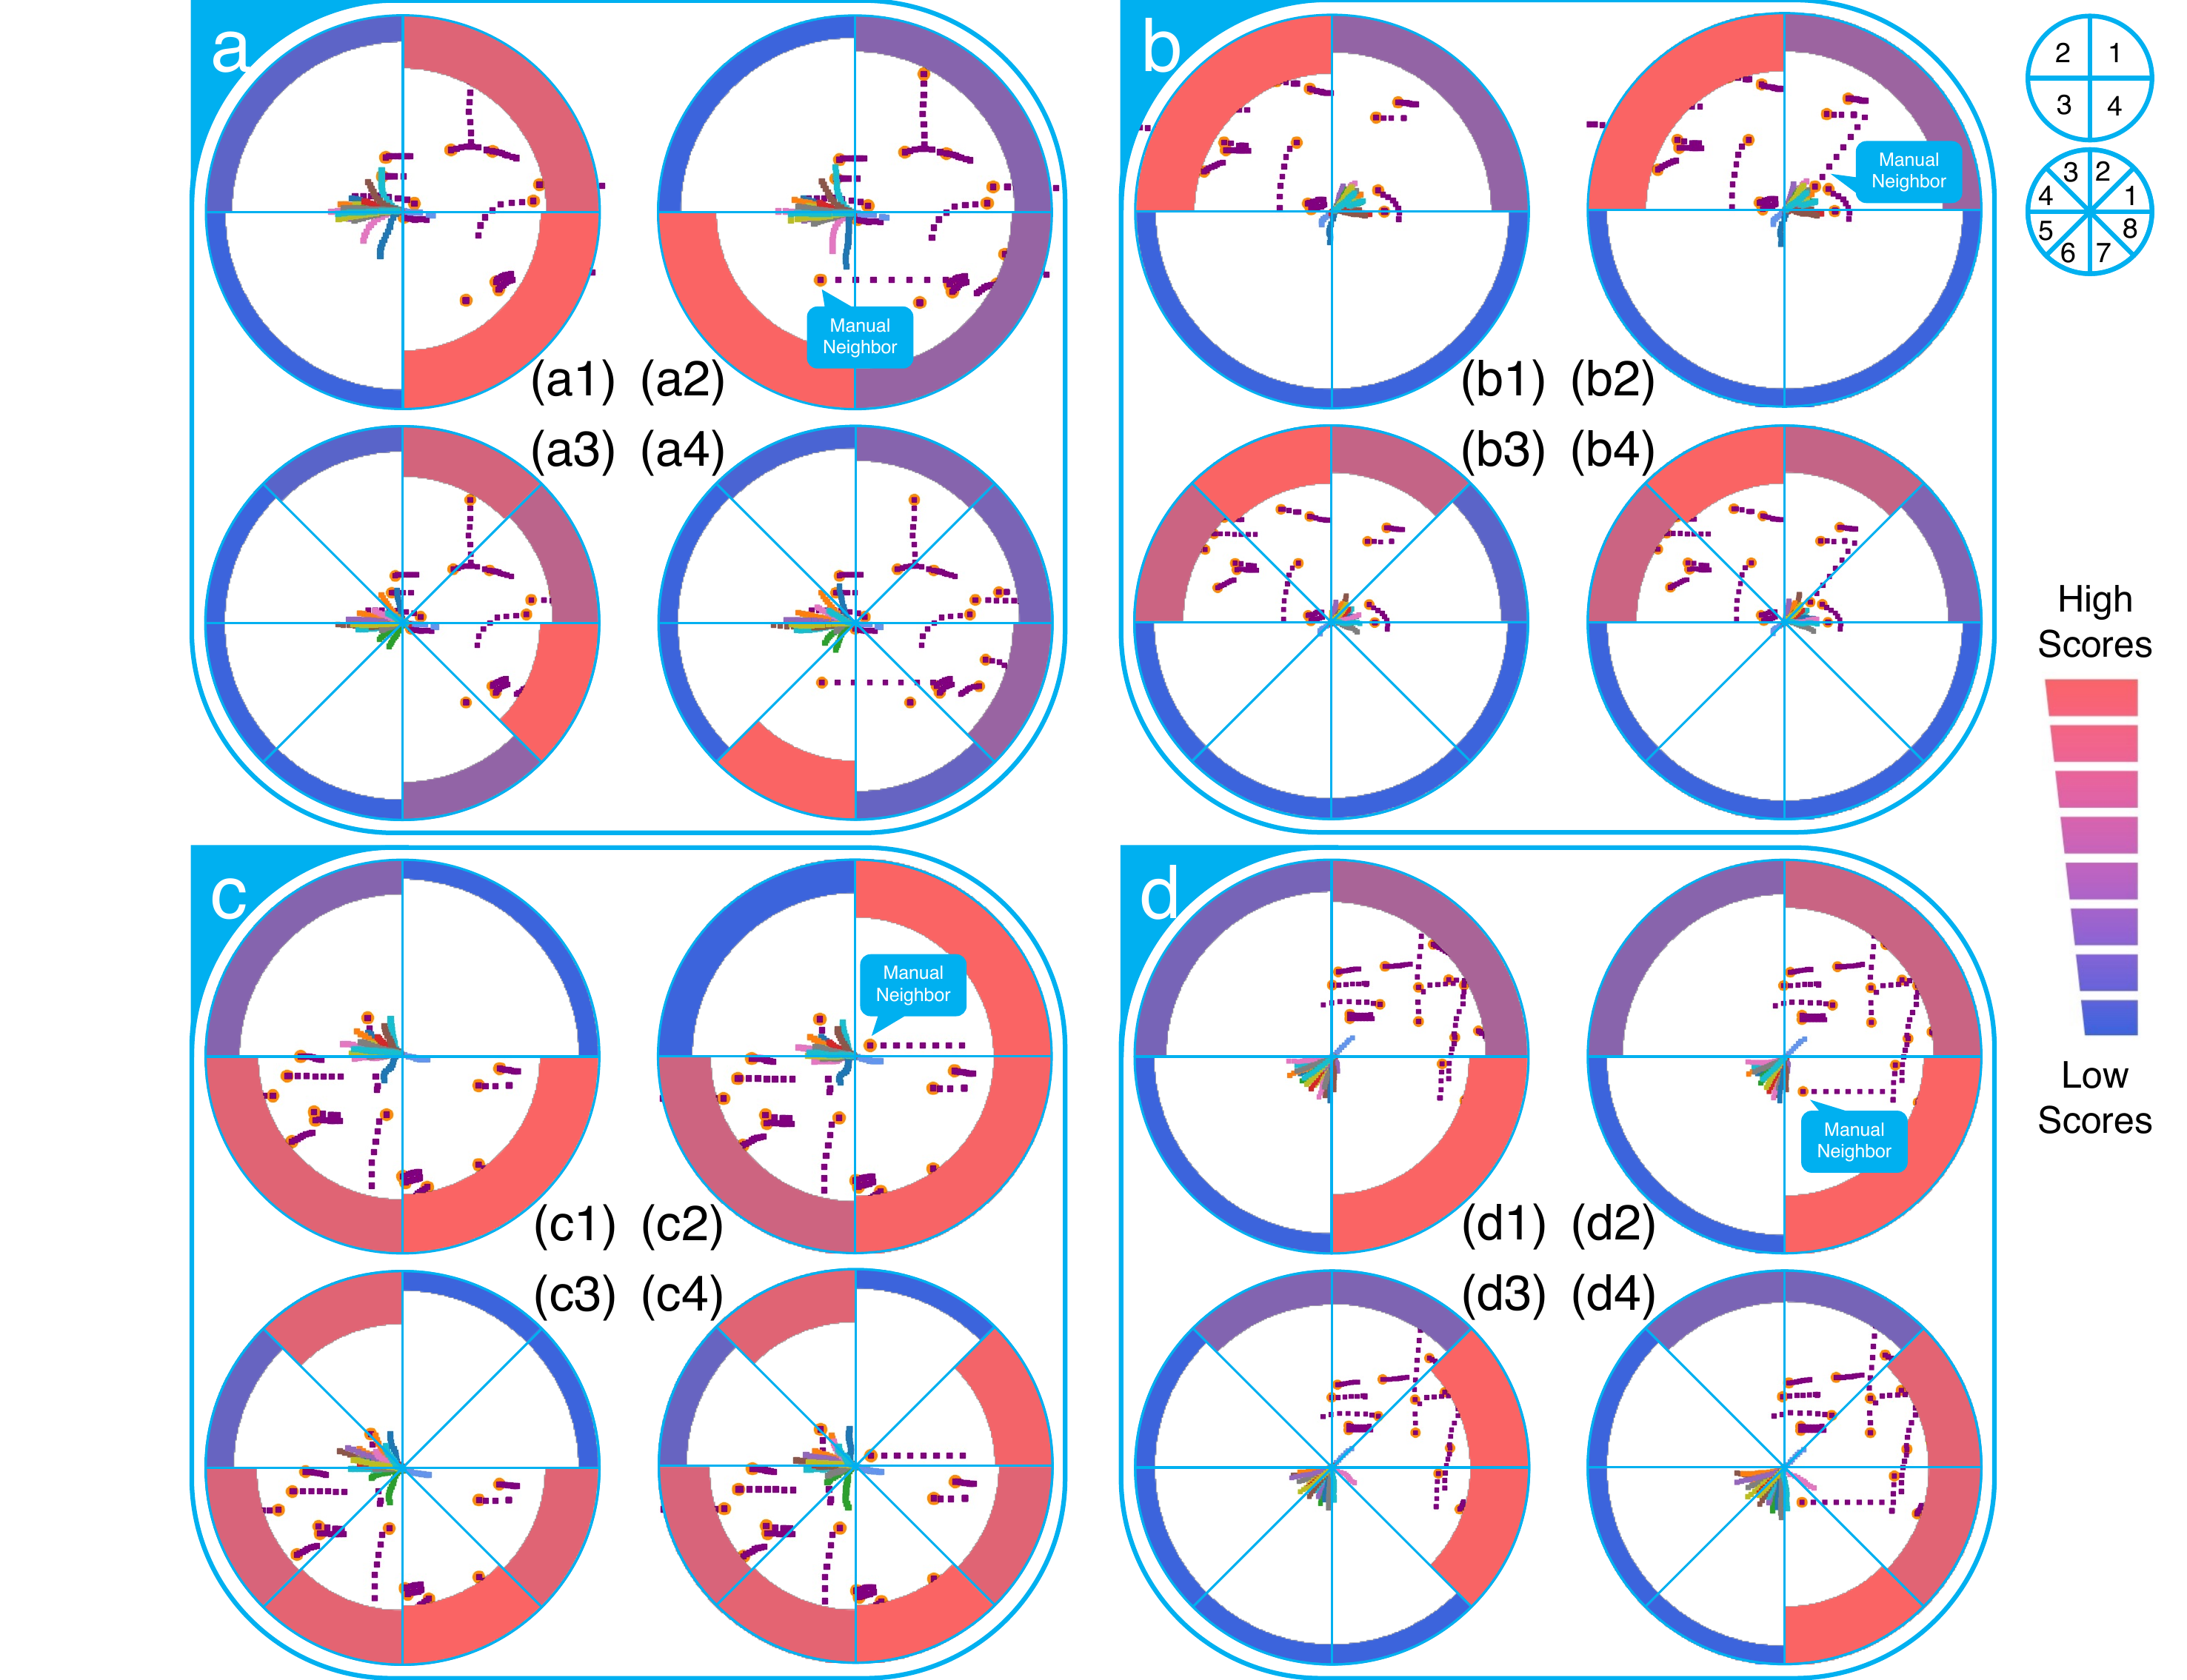}
    \caption{
        Visualized predicted trajectories and the corresponding attention scores of several real-world cases by adding additional manual neighbors.
        For each case $x \in \{\textrm{a, b, c, d}\}$, subfigure ($x$1) is the \textbf{4-partition} ($N_\theta = 4$) model's prediction, and ($x$3) is \textbf{8-partition} ($N_\theta = 8$) prediction.
        subfigures ($x$2) and ($x$4) are obtained by adding manual neighbors to cases ($x$1) and ($x$3), respectively.
    }
    \label{fig_attention_partitions_toy}
\end{figure*}

\subsection{Quantitative Analyses}

We run ablation experiments to validate how the number of \MODEL~partitions $N_\theta$ affects models' quantitative performance.
In \TABLE{tab_ab_partitions}, 8-partition \MODEL~models perform the best, outperforming 4-partition variations for about 1.1\% to 1.8\% ADE and FDE.
Especially, models with $N_\theta = 1$ work even worse, including up to 2.5\% ADE drop compared to 4-partitions'.
Comparing \VMODEL~and \VMODEL-SC-a4, we find that the latter one even has about 0.1 pixels worse FDE.
It aligns with our intuition that the more partitions the higher resolutions for describing social behaviors.
While vice versa, too few partitions may lead to a coarse description of interactions, even mislead the model, thus significantly reducing prediction performance.

Note that due to the settings of predicting trajectories based on 8 historical observed frames on SDD, the maximum number of partitions is set to 8 to prevent unnecessary zero-paddings in trajectories' representations from pulling down the performance of the original backbone trajectory prediction network.
To verify this thought, we expand the \MODEL~to make it available to handle $N_\theta > t_h$ cases by zero-padding trajectory representations (\IE, the $\mathbf{f}^i_{\mathrm{traj}}$ in Eq. (13)).
Results of variations with postfixes \{a6, a7, a8\} reported in \TABLE{tab_ab_partitions} are obtained under this new setting.
In addition, we have attached the loss curves and metrics curves of these $N_\theta > t_h$ variations in \FIG{fig_loss_partitions}.
It shows that the loss may drop faster as the $N_\theta$ raises, but simultaneously exacerbates the risk of overfitting.
We can further infer that even though a higher $N_\theta$ may provide better results, it also compresses the information in trajectories while reducing training stability.
On balance, $N_\theta = 8$ may be a good compromise (ETH-UCY and SDD).
As a result, we regard that $N_\theta$ should be no more than the $t_h$ in the main paper.

\subsection{Qualitative Analyses}

\FIG{fig_attention_partitions} provides the visualized attention scores in different prediction cases on SDD-little0 with the $N_\theta = 4$ (subfigures (a1) to (a5)) and the $N_\theta = 8$ ((b1) to (b5)) \EVMODEL-SC models.
These two models are trained and validated under the same condition except for the $N_\theta$.

Comparing \FIG{fig_attention_partitions} (a3) and (b3), the 8-partition model provides trajectories with different social behaviors for $\theta \in \left[1.5\pi, 2\pi\right)$, \IE, partitions 7 and 8.
In detail, predictions in partition-8 mostly try to avoid the right-coming neighbor, while predictions in partition-7 mostly walk as normal cases.
For the 4-partition model's predictions in \FIG{fig_attention_partitions} (a3), predictions within the whole partition-4 all present the avoidance tendance, even though some predicted trajectories are far away from the existing neighbors.
Similar cases also appear in cases (a2, partition-4) v.s. (b2, partitions 7 and 8) and cases (a5, partition-3) v.s. (b5, partitions 5 and 6).
All these comparisons point out that a smaller number of \MODEL~partitions may lead to a coarser recognition and modeling of social behaviors, thus further causing misleading shifts in the predicted trajectories.

% \textbf{Toy Examples with Different $N_\theta$.}
We also add manual neighbors to real-world prediction cases on SDD-little0 to validate both $N_\theta = 4$ and $N_\theta = 8$ \EVMODEL-SC models' responses.
As shown in \FIG{fig_attention_partitions_toy}, $N_\theta = 8$ model presents better spatial resolutions for handling social interactions.
For example, compared to the $N_\theta = 4$ case (c2, partition-1), the corresponding $N_\theta = 8$ partition (c4, partition-2) has been less affected due to the manual neighbor.
As a result, predictions in 8-partitions cases \{(c4, partition-3), (c4, partition-4)\} show different interactive trends.
These results indicate that 8-partition \MODEL~models have better angular resolution to model potential social interactions as well as quantify their roles in modifying forecast results.

\end{document}
