# Supplementary material for: SocialCircle+: Learning the Angle-based Conditioned Interaction Representation for Pedestrian Trajectory Prediction
Source: arXiv:2409.14984 source file (2024-09-23)
Supplement: Supplementary file 3 [file s3f1_attention_partitions.tex]

%%%%%%%%%%%%%%%%%%%%%%%
%% Author: Beihao Xia
%% Date: 2023-09-27 16:34:05
%% LastEditors: Conghao Wong
%% LastEditTime: 2023-10-08 20:59:37
%% Description: file content
%% Github: https://cocoon2wong.github.io
%% Copyright 2023 Beihao Xia, All Rights Reserved.
%%%%%%%%%%%%%%%%%%%%%%%

\documentclass[../../paper.tex]{subfiles}

\begin{document}

\begin{figure*}[t]
    \centering
    \includegraphics[width=1.0\linewidth]{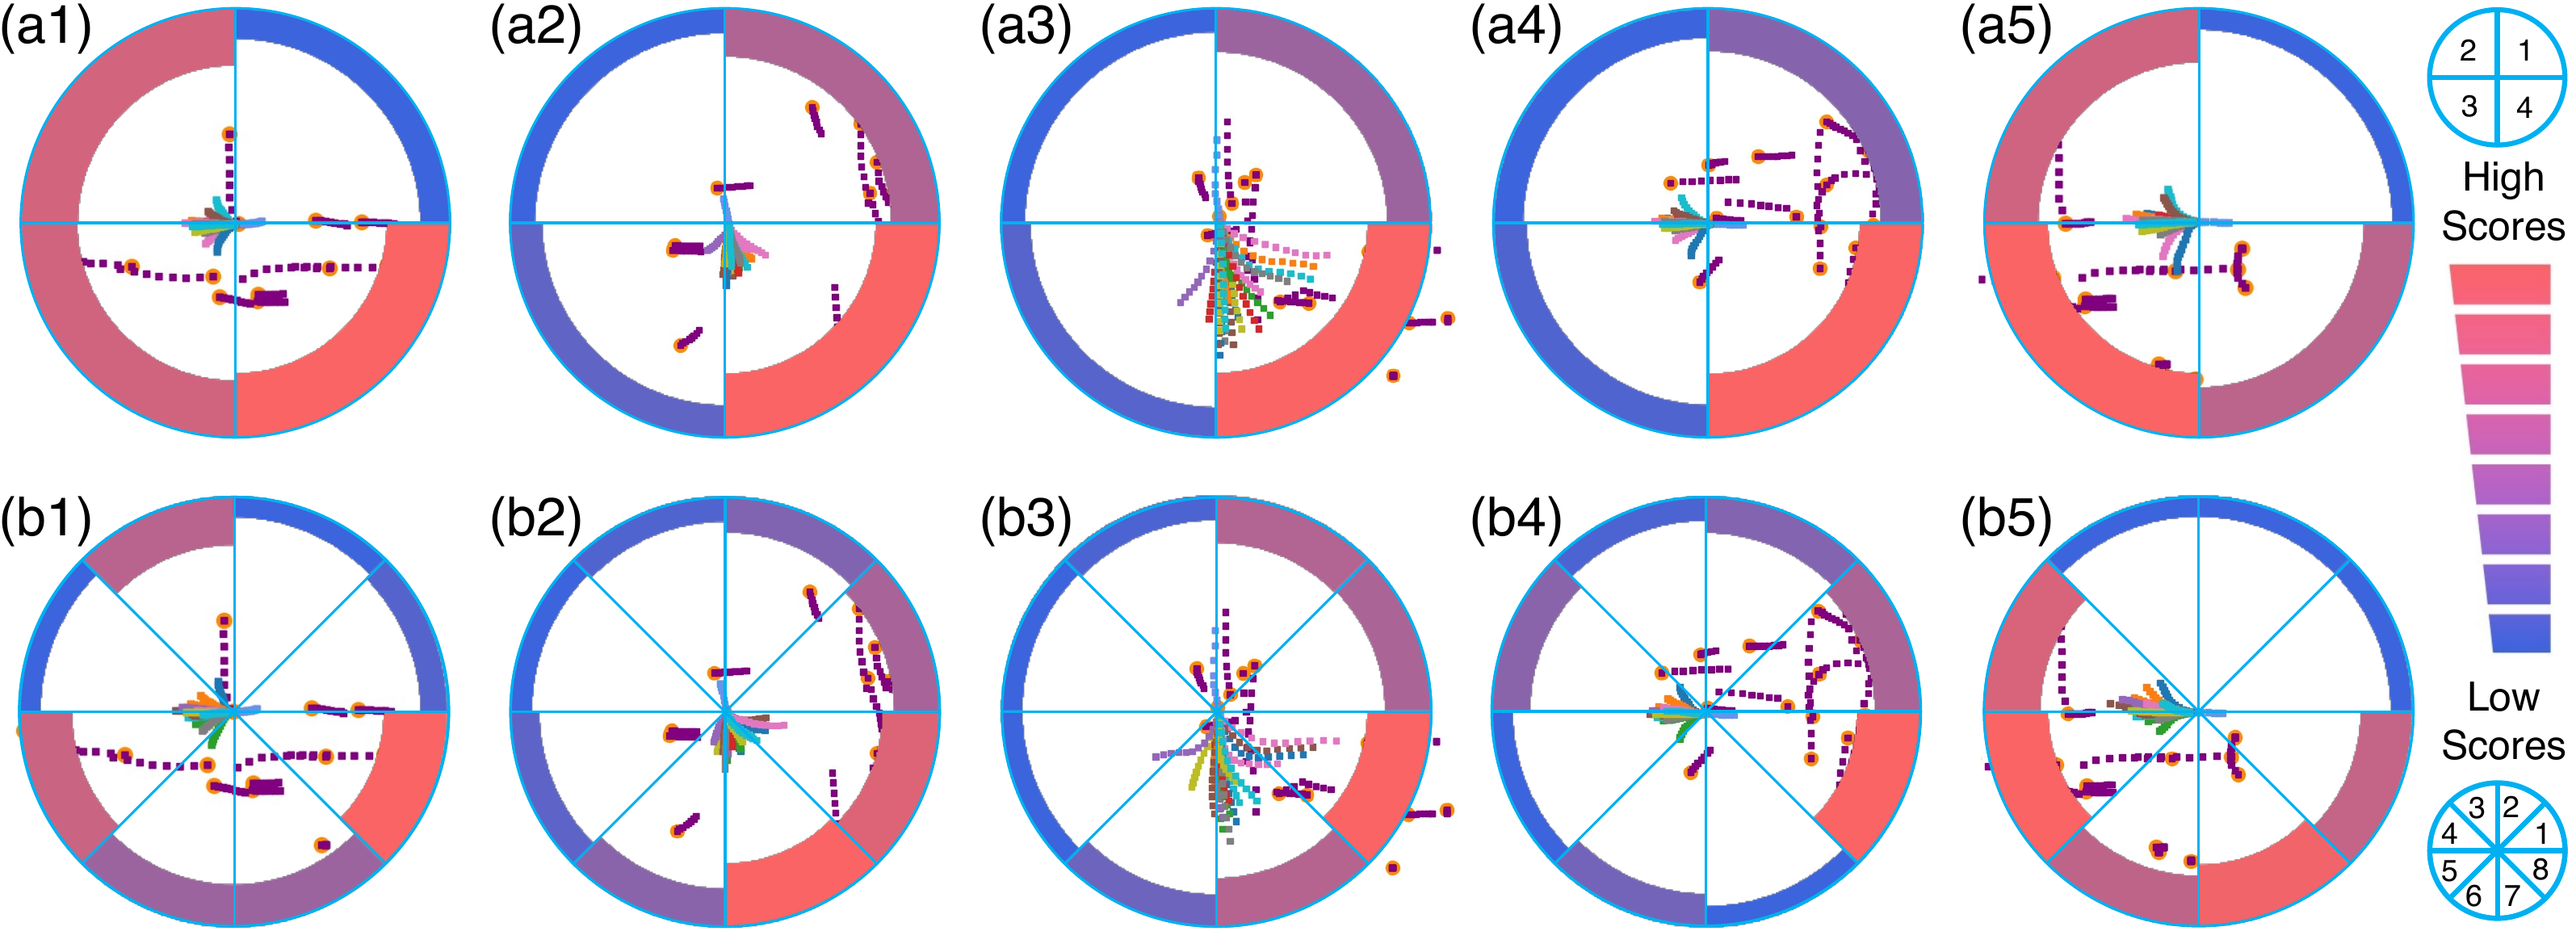}
    \caption{
        Visualized predicted trajectories and the corresponding attention scores of several real-world prediction cases on SDD-little0 provided by the \textbf{4-partition} \EVMODEL-SC (a1) to (a5) and the \textbf{8-partition} \EVMODEL-SC (b1) to (b5).
    }
    \label{fig_attention_partitions}
\end{figure*}

\end{document}
