# Supplementary material for: SocialCircle+: Learning the Angle-based Conditioned Interaction Representation for Pedestrian Trajectory Prediction
Source: arXiv:2409.14984 source file (2024-09-23)
Supplement: Supplementary file 4 [file s3f2_attention_partitions_toy.tex]

%%%%%%%%%%%%%%%%%%%%%%%
%% Author: Conghao Wong
%% Date: 2023-09-26 21:26:28
%% LastEditors: Beihao Xia
%% LastEditTime: 2023-10-08 10:04:46
%% Description: file content
%% Github: https://cocoon2wong.github.io
%% Copyright 2023 Conghao Wong, All Rights Reserved.
%%%%%%%%%%%%%%%%%%%%%%%

\documentclass[../../paper.tex]{subfiles}

\begin{document}

\begin{figure*}[t]
    \centering
    \includegraphics[width=0.916\linewidth]{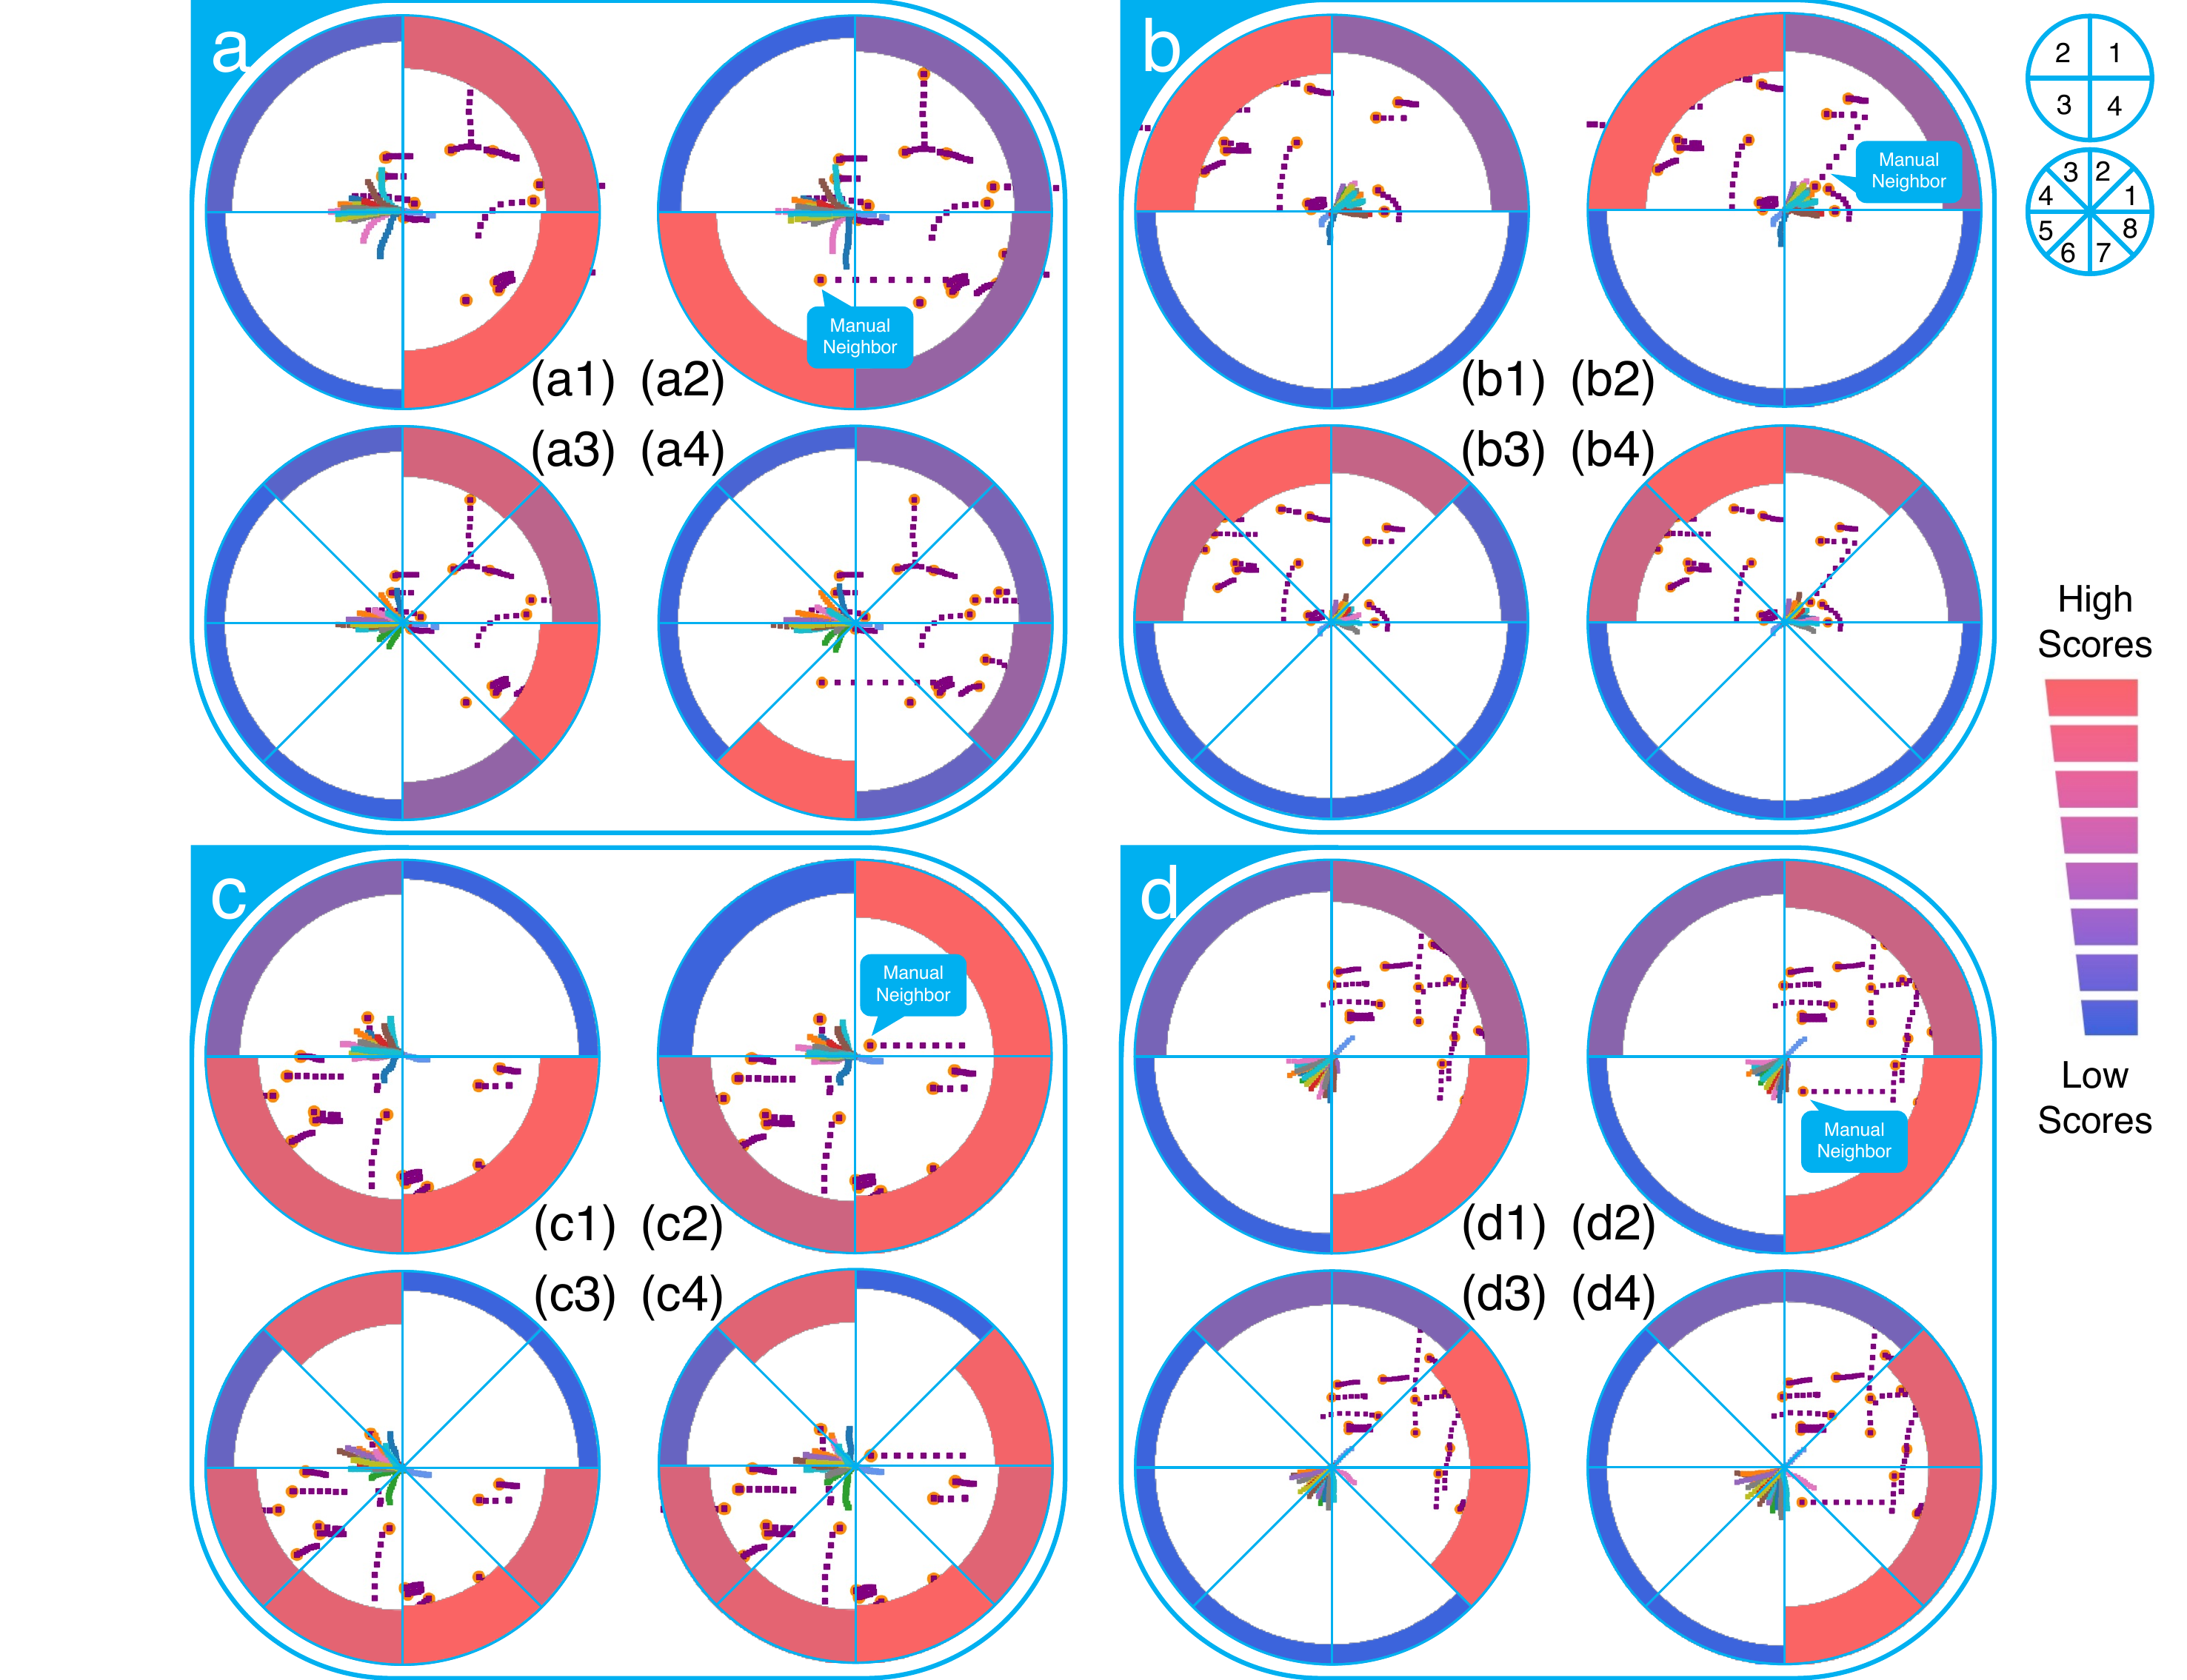}
    \caption{
        Visualized predicted trajectories and the corresponding attention scores of several real-world cases by adding additional manual neighbors.
        For each case $x \in \{\textrm{a, b, c, d}\}$, subfigure ($x$1) is the \textbf{4-partition} ($N_\theta = 4$) model's prediction, and ($x$3) is \textbf{8-partition} ($N_\theta = 8$) prediction.
        subfigures ($x$2) and ($x$4) are obtained by adding manual neighbors to cases ($x$1) and ($x$3), respectively.
    }
    \label{fig_attention_partitions_toy}
\end{figure*}

\end{document}
