# Supplementary material for: SocialCircle+: Learning the Angle-based Conditioned Interaction Representation for Pedestrian Trajectory Prediction
Source: arXiv:2409.14984 source file (2024-09-23)
Supplement: Supplementary file 5 [file s3f3_loss_partitions.tex]

%%%%%%%%%%%%%%%%%%%%%%%
%% Author: Conghao Wong
%% Date: 2023-09-26 21:26:28
%% LastEditors: Conghao Wong
%% LastEditTime: 2024-03-13 20:31:19
%% Description: file content
%% Github: https://cocoon2wong.github.io
%% Copyright 2023 Conghao Wong, All Rights Reserved.
%%%%%%%%%%%%%%%%%%%%%%%

\documentclass[../../paper.tex]{subfiles}

\begin{document}

\begin{figure}[t]
    \centering
    \includegraphics[width=1.0\linewidth]{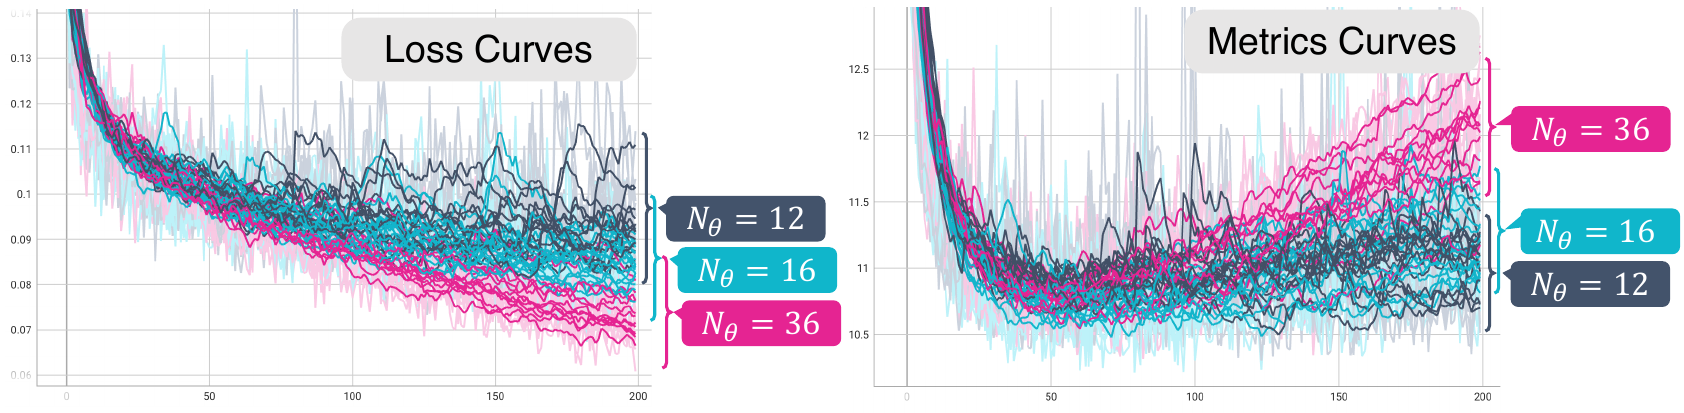}
    \caption{
        Loss curves (left, $\ell_2$ loss) and metrics curves (right, ADE) of \EVMODEL-SC variations a6 to a8 ($N_\theta \in \{12, 16, 36\}$).
    }
    \label{fig_loss_partitions}
\end{figure}

\end{document}
