# Supplementary material for: SocialCircle+: Learning the Angle-based Conditioned Interaction Representation for Pedestrian Trajectory Prediction
Source: arXiv:2409.14984 source file (2024-09-23)
Supplement: Supplementary file 6 [file s3t1_ab_partition.tex]

%%%%%%%%%%%%%%%%%%%%%%%
%% Author: Conghao Wong
%% Date: 2023-08-21 15:33:41
%% LastEditors: Conghao Wong
%% LastEditTime: 2024-03-18 10:59:00
%% Description: file content
%% Github: https://cocoon2wong.github.io
%% Copyright 2023 Conghao Wong, All Rights Reserved.
%%%%%%%%%%%%%%%%%%%%%%%

\documentclass[../../paper.tex]{subfiles}

\begin{document}

\begin{table}[tbp]
    \small
    \centering
    \begin{tabular}{c|c|cc}
        \toprule
        Variations
        & $N_\theta$
        & ADE/FDE
        & Gain (\%) \\

        \midrule
        \VMODEL* & - & 7.04/10.94 & -4.92\%/-2.63\% \\
        \VMODEL-SC-a4 & 1 & 6.96/11.05 & -3.73\%/-3.66\% \\
        \VMODEL-SC-a5 & 4 & 6.79/10.80 & -1.19\%/-1.31\% \\
        \VMODEL-SC & 8 & 6.71/10.66 & (base) \\
        \VMODEL-SC-a6 & 12 & 6.65/10.60 & +0.89\%/+0.56\%\\
        \VMODEL-SC-a7 & 16 & 6.68/10.65 & +0.45\%/+0.09\%\\
        \VMODEL-SC-a8 & 36 & 6.64/10.64 & +1.04\%/+0.19\%\\

        \midrule
        \EVMODEL* & - & 6.73/10.75 & -2.91\%/-3.76\% \\
        \EVMODEL-SC-a4 & 1 & 6.66/10.70 & -1.83\%/-3.28\% \\
        \EVMODEL-SC-a5 & 4 & 6.61/10.55 & -1.07\%/-1.83\% \\
        \EVMODEL-SC & 8 & 6.54/10.36 & (base) \\
        \EVMODEL-SC-a6 & 12 & 6.50/10.34 & +0.61\%/+0.19\% \\
        \EVMODEL-SC-a7 & 16 & 6.46/10.22 & +1.22\%/+1.35\% \\
        \EVMODEL-SC-a8 & 36 & 6.57/10.41 & -0.46\%/-0.48\% \\
        
        \bottomrule
    \end{tabular}
    \caption{
        Ablation studies on verifying the number of \MODEL~partitions $N_\theta$ with different backbone models on SDD.
        Values in the ``Gain'' column are the percentage ADE and FDE gain compared to the base 8-partition model (denoted with ``(base)'').
    }
    \label{tab_ab_partitions}
\end{table}

\end{document}
