# Supplementary material for: SocialCircle+: Learning the Angle-based Conditioned Interaction Representation for Pedestrian Trajectory Prediction
Source: arXiv:2409.14984 source file (2024-09-23)
Supplement: Supplementary file 7 [file s4f1_factor_vis.tex]

%%%%%%%%%%%%%%%%%%%%%%%
%% Author: Ziqian Zou
%% Date: 2023-11-20 17:21:13
%% LastEditors: Ziqian Zou
%% LastEditTime: 2024-03-22 16:20:43
%% Description: file content
%% Github: https://github.com/LivepoolQ
%% Copyright 2023 Ziqian Zou, All Rights Reserved.
%%%%%%%%%%%%%%%%%%%%%%%

\documentclass[../../paper.tex]{subfiles}

\begin{document}

\begin{figure*}[t]
    \centering
    \includegraphics[width=1.0\linewidth]{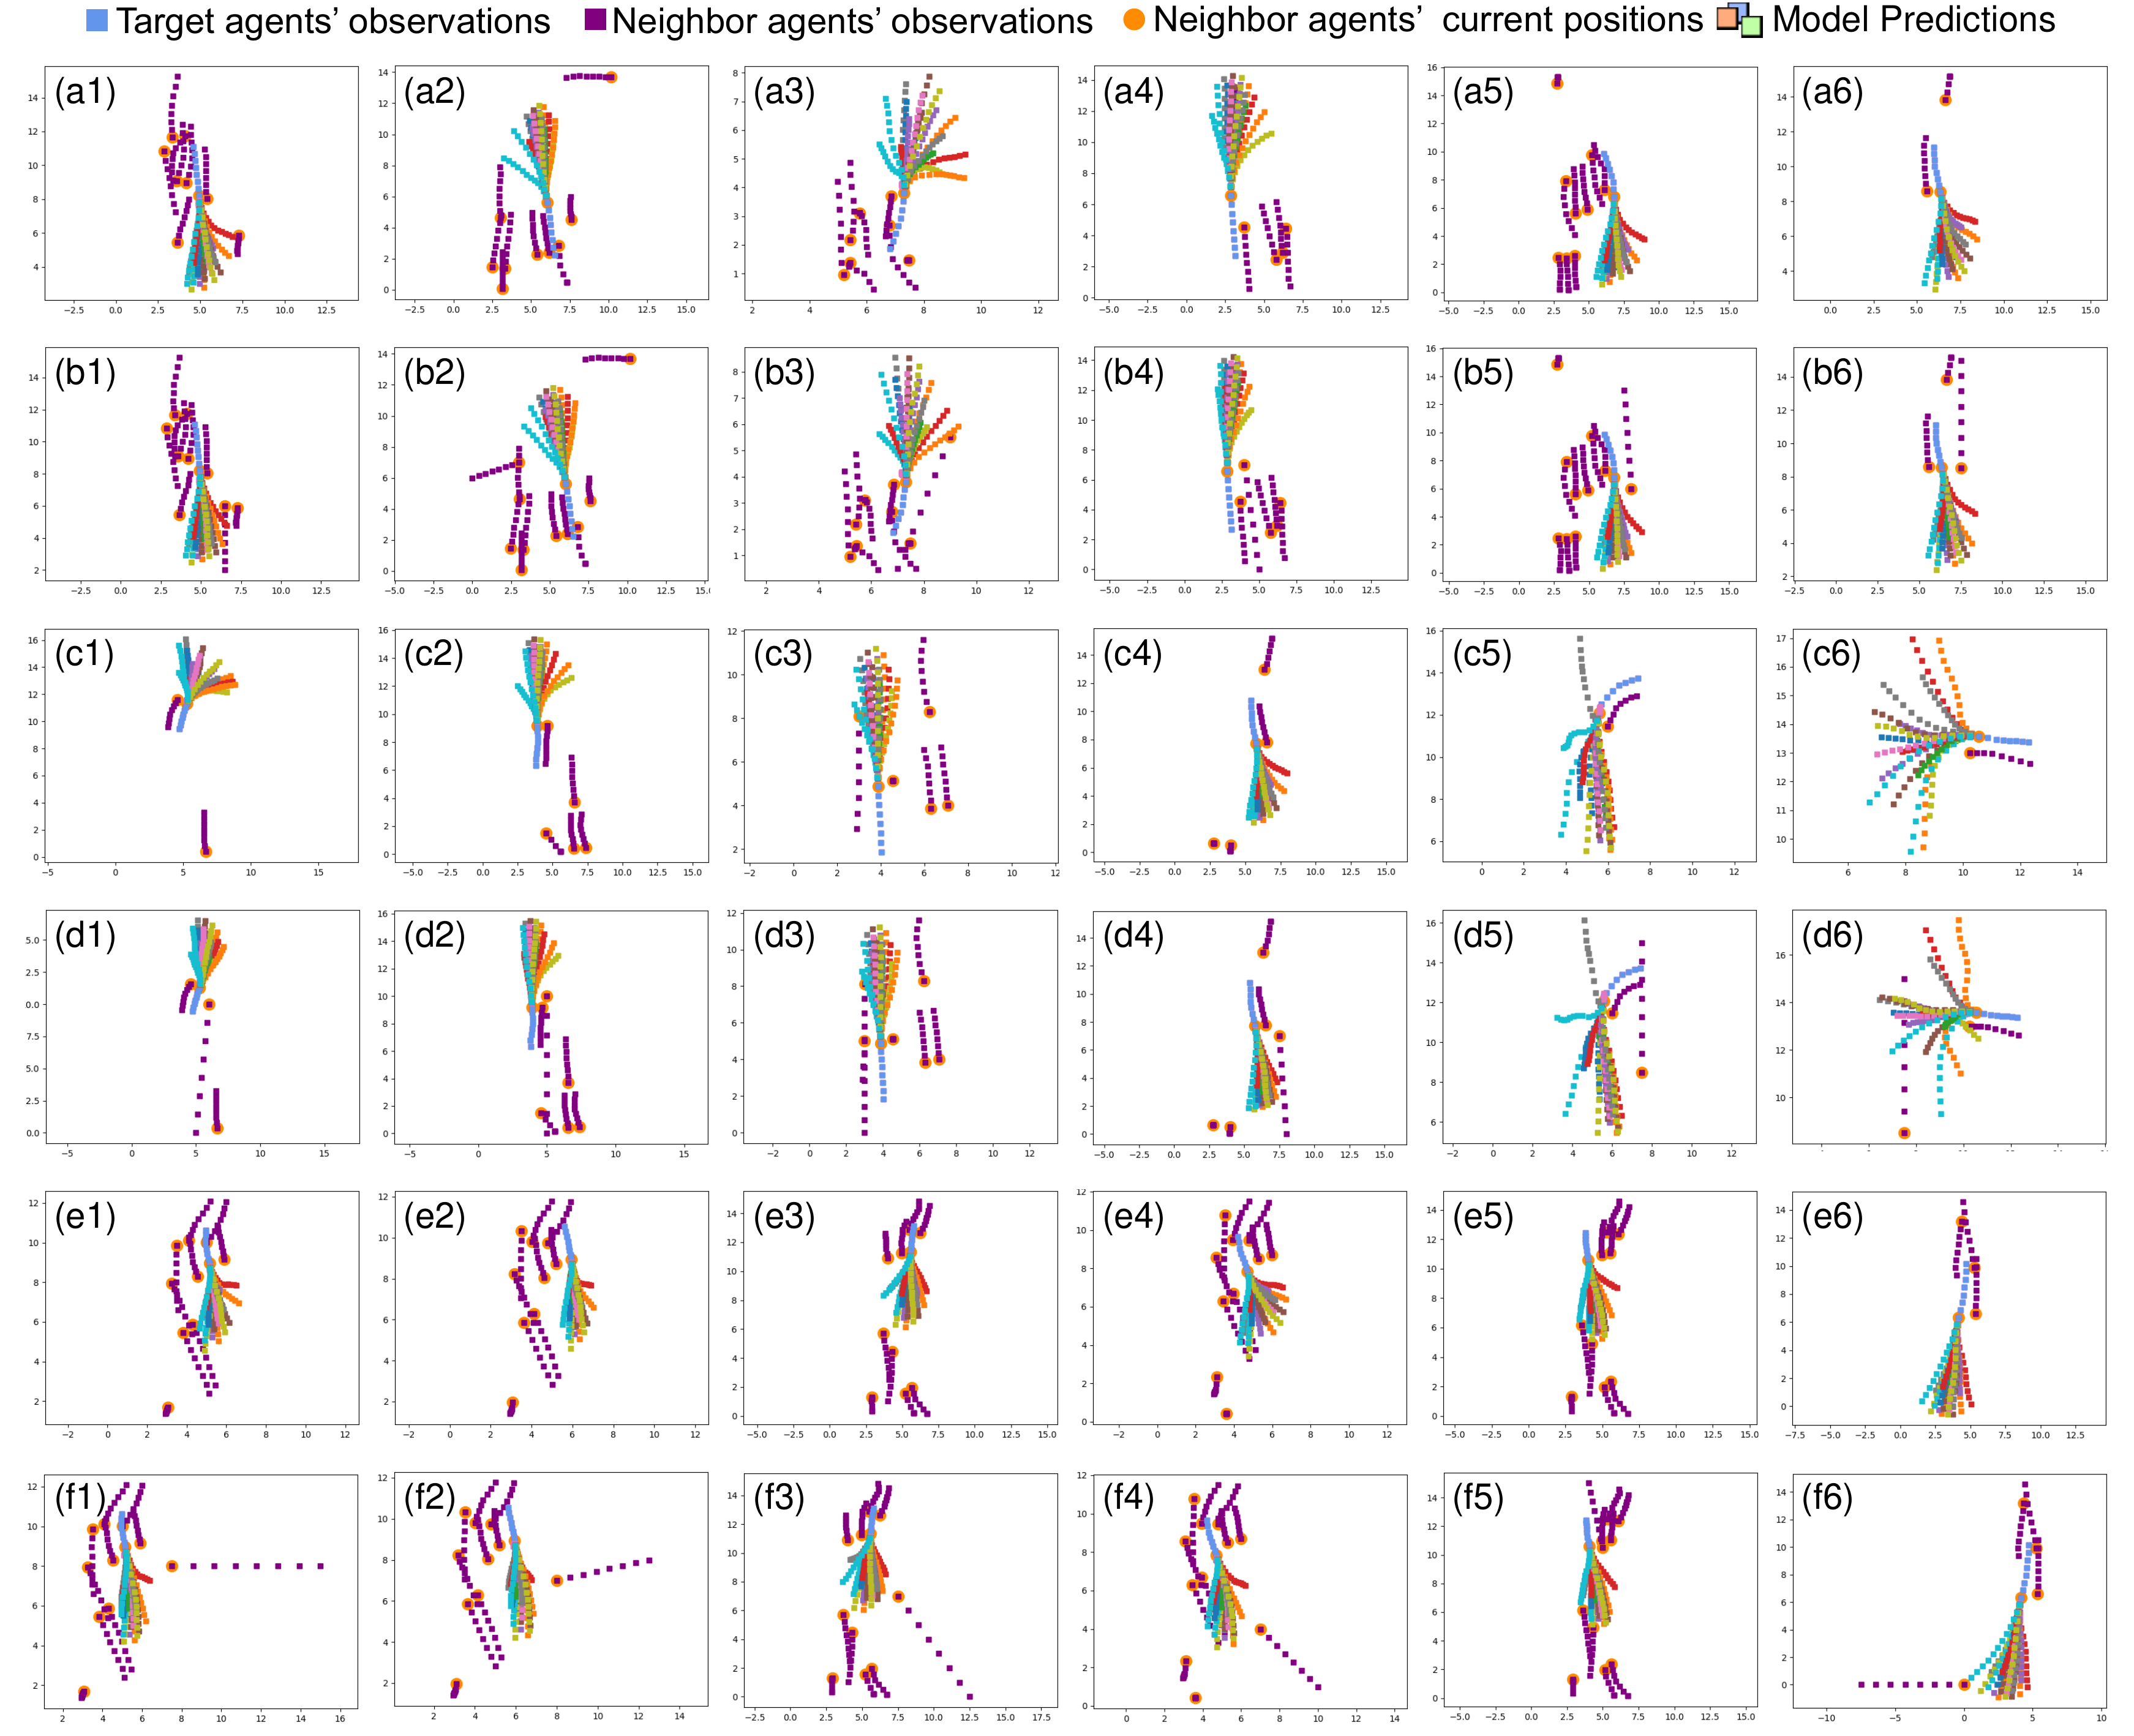}
    \caption{
        Toy examples (linear interpolation) on validating the effectiveness of the overall modification of social interactions.
        We add manual neighbors to the original ETH-UCY prediction scenes and visualize how they change the predicted trajectories.
        Prediction case in subfigure ($xn$), where $x \in \{\textrm{a, c, e}\}, n\in\{1, 2, 3, 4, 5, 6\}$, represents the original prediction scene in UCY-zara1, and the corresponding ($yn, y \in \{\textrm{b, d, f}\}$) case represents prediction considering the manual neighbor.
    }
    \label{fig_factor_vis}
\end{figure*}

\end{document}
