# Supplementary material for: SocialCircle+: Learning the Angle-based Conditioned Interaction Representation for Pedestrian Trajectory Prediction
Source: arXiv:2409.14984 source file (2024-09-23)
Supplement: Supplementary file 8 [file s4f2_curve_neighbor.tex]

%%%%%%%%%%%%%%%%%%%%%%%
%% Author: Ziqian Zou
%% Date: 2024-03-19 20:57:59
%% LastEditors: Beihao Xia
%% LastEditTime: 2024-03-26 15:46:50
%% Description: file content
%% Github: https://github.com/LivepoolQ
%% Copyright 2024 Ziqian Zou, All Rights Reserved.
%%%%%%%%%%%%%%%%%%%%%%%
\documentclass[../../paper.tex]{subfiles}

\begin{document}

\begin{figure*}[t]
    \centering
    \includegraphics[width=1.0\linewidth]{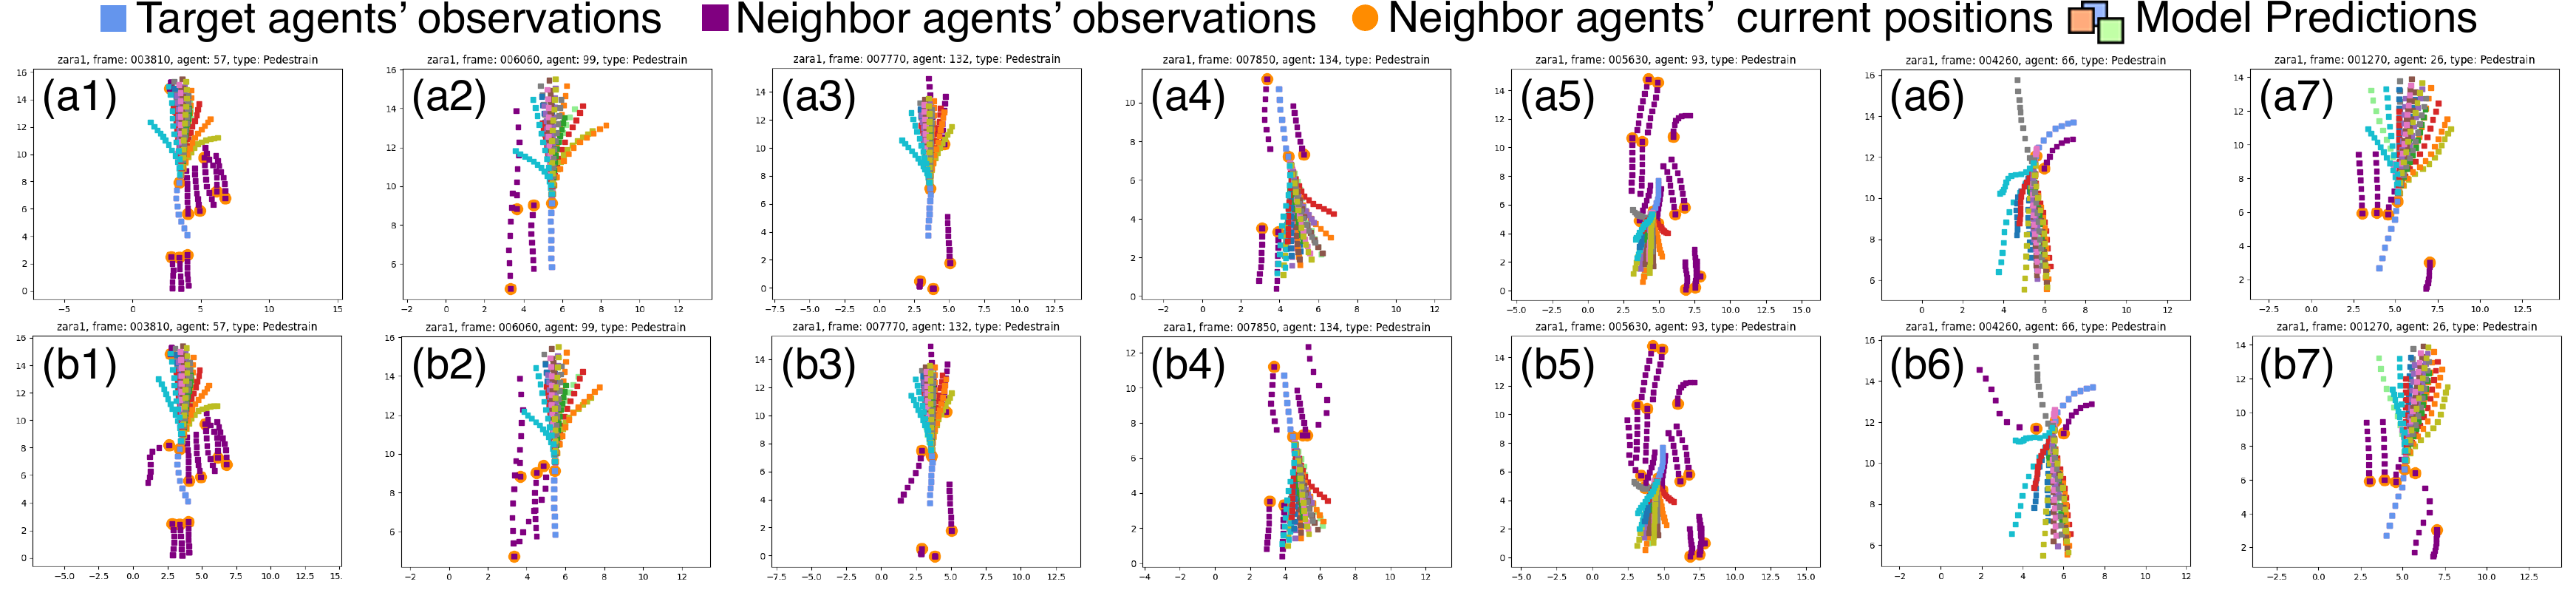}
    \caption{
        Toy example (linear-velocity interpolation) on validating social interactions.
        Compared to the linearly-interpolated trajectories, we add several non-linear patterns to the trajectories of manual neighbors to further reflect their fine-level motions. 
        The prediction case in subfigure (a$n$), where $n\in\{1, 2, 3, 4, 5, 6, 7\}$, represents the original prediction scene in UCY-zara1, and the corresponding (b$n$) case represents prediction considering the curved-moving manual neighbor.
    }
    \label{fig_curve_neighbor}
\end{figure*}

\end{document}
