# Supplementary material for: SocialCircle+: Learning the Angle-based Conditioned Interaction Representation for Pedestrian Trajectory Prediction
Source: arXiv:2409.14984 source file (2024-09-23)
Supplement: Supplementary file 9 [file s5_components.tex]

%%%%%%%%%%%%%%%%%%%%%%%
%% Author: Conghao Wong
%% Date: 2024-07-18 15:32:01
%% LastEditors: Conghao Wong
%% LastEditTime: 2024-07-19 16:59:18
%% Github: https://cocoon2wong.github.io
%% Copyright 2024 Conghao Wong, All Rights Reserved.
%%%%%%%%%%%%%%%%%%%%%%%

\documentclass[../../paper.tex]{subfiles}

\begin{document}

\section{Additional Experimental Analyses on Circle Meta Components}
\label{sec_appendix_components}

\TODO{3个主成分对于预测的贡献，fc层}

\end{document}
